# Supplementary material for: A new class of metrics for learning on real-valued and structured data
Source: arXiv:1603.06846 source file (2018-04-23)
Supplement: Supplementary file 1 [file main_appendix.tex]

\documentclass[twoside,leqno,twocolumn]{article}
\usepackage{ltexpprt}

%%%%%%%%%%%%%%%%%%%%%%%%%%%%%%%%%%%%%%%%%%%%%%%%%%%%%%%%%%%%%%%%%%
%%%%%%%% our own packages %%%%%%%%%%%%%%%%%
%%%%%%%%%%%%%%%%%%%%%%%%%%%%%%%%%%%%%%%%%%%%%%%%%%%%%%%%%%%%%%%%%%

\usepackage{booktabs} % For formal tables

%%% Load packages
% \usepackage{algcompatible,amssymb,amsmath,amsthm,amscd}
% \usepackage{amssymb,amsmath,amsthm,amscd} debugging
\usepackage{amssymb,amsmath,amscd}

\usepackage{graphicx}

\usepackage{epsfig}
\usepackage{bm}
\usepackage{mathtools}
\usepackage{color}
\usepackage{nicefrac}

%%% Additional packages
\usepackage{lmodern}
\usepackage{multirow}
\usepackage{bbm}
\usepackage{units}
\usepackage{url}
\usepackage{longtable}
\usepackage{color}

\usepackage[english]{babel}
\usepackage{csquotes}

%%% for the Venn diagram
\usepackage{tikz}
\tikzset{fontscale/.style = {font=\relsize{11pt}}}
\usetikzlibrary{decorations.markings}

%%% Mathematical terms
\usepackage{latexsym}

\AtBeginDocument{}

%%%%%%%%%%%%%%%%%%%%%%%%%%%%%%%%%%%%%%%%%%%%%%%%%%%%%%%%%%%%%%%%%%
%%%%%%%% our own packages %%%%%%%%%%%%%%%%%
%%%%%%%%%%%%%%%%%%%%%%%%%%%%%%%%%%%%%%%%%%%%%%%%%%%%%%%%%%%%%%%%%%

\begin{document}

\title{Appendix}
% \author{Ruiyu Yang, Yuxiang Jiang, Scott Mathews, \\ \and Matthew W. Hahn, Elizabeth A. Housworth, Predrag Radivojac \\ \and Indiana University, Bloomington, Indiana, U.S.A.}
%\thanks{Indiana University, Bloomington, Indiana, U.S.A.}}
% \title{A new class of metrics for learning on real-valued and structured data}
% \author{Ruiyu Yang, Yuxiang Jiang, Scott Mathew, Matthew W. Hahn, Elizabeth A. Housworth, Predrag Radivojac\thanks{Indiana University} \\
% \and
% Tricia Manning\thanks{Society for Industrial and Applied Mathematics.}}
\date{}

\maketitle

% Copyright Statement
% When submitting your final paper to a SIAM proceedings, it is requested that you include
% the appropriate copyright in the footer of the paper.  The copyright added should be 
% consistent with the copyright selected on the copyright form submitted with the paper.
% Please note that "20XX" should be changed to the year of the meeting.

% Default Copyright Statement
\fancyfoot[R]{\footnotesize{\textbf{Copyright \textcopyright\ 2018 by SIAM\\
Unauthorized reproduction of this article is prohibited}}}

% Depending on which copyright you agree to when you sign the copyright form, the copyright 
% can be changed to one of the following after commenting out the default copyright statement
% above.

%\fancyfoot[R]{\footnotesize{\textbf{Copyright \textcopyright\ 20XX\\
%Copyright for this paper is retained by authors}}}

%\fancyfoot[R]{\footnotesize{\textbf{Copyright \textcopyright\ 20XX\\
%Copyright retained by principal author's organization}}}

%\pagenumbering{arabic}
%\setcounter{page}{1}%Leave this line commented out.

\maketitle

\input{appendix.tex}
\end{document}
